# Supplementary material for: Uncertainty-aware INVASE: Enhanced Breast Cancer Diagnosis Feature Selection
Source: arXiv:2105.02693 source file (2021-05-04)
Supplement: Supplementary file 1 [file Appendix.pdf]

# Appendix
# Uncertainty-aware INVASE: Enhanced Breast Cancer Diagnosis Feature Selection*

**Jia-Xing Zhong,**[1] **Hongbo Zhang** [2]
[1] Department of Computer Science, University of Oxford
[2] Department of Computer and Information Sciences, Virginia Military Institute
jiaxing.zhong@cs.ox.ac.uk, hbzhang@vt.edu

## 1 Detailed Analysis on the Equivalency between our Model with $\sigma^2 \to 0$ and the vanilla INVASE

The differences between the vanilla INVASE and ours are based on two new modules: uncertainty quantification and reward shaping. To analyze the equivalency, *all we need to do is to prove the equivalency w.r.t. those two components*.

**Uncertainty Quantification** In our model, we treat data as samples from learnable uncertainty-aware distributions as shown in Equation (5):

$$P_D(y|\mathbf{x},\mathbf{s}) = P^{\psi}(y - f^{\phi}(\mathbf{x},\mathbf{s}))\,.$$

where $P_D(y|\mathbf{x},\mathbf{s}) \sim N(\mu,\sigma^2)$ in our model. We should prove the Gaussian distribution approaches to a Dirac delta function when $\sigma^2 \to 0$. Given a Gaussian distribution $N(\mu,\sigma^2)$, the probability density function of a variable $t$ is:

$$f(t;\mu,\sigma) = \frac{1}{\sigma\sqrt{2\pi}}\exp(-\frac{(t-\mu)^2}{2\sigma^2})\,.$$

Hence,

$$\lim_{\sigma^2\to 0} f(t;\mu,\sigma) = \begin{cases} \infty & (t=\mu) \\ 0 & (t \neq \mu) \end{cases}\,,$$

where $\int f(t;\mu,\sigma)dt = 1$ according to the characteristics of a probability density function. By definition, $\delta(t-\mu) = \lim_{\sigma^2\to 0} f(t;\mu,\sigma)$.

**Reward Shaping** In Equation (10), the total reward is defined as:

$$R(\mathbf{x},\mathbf{s}) = \omega\sigma^2(\mathbf{x},\mathbf{s};\psi) - \hat{l}(\mathbf{x},\mathbf{s}) - \lambda||\mathbf{s}||_0\,,$$

if $\sigma^2(\mathbf{x},\mathbf{s};\psi) \to 0$, then $R(\mathbf{x},\mathbf{s}) \to -\hat{l}(\mathbf{x},\mathbf{s}) - \lambda||\mathbf{s}||_0$. That is just the form of Equation (9), so they are equivalent.

Therefore, the vanilla INVASE is a *particular case* of our uncertainty-aware INVASE. When the variance $\sigma^2 \to 0$, the Gaussian distribution $N(\mu,\sigma^2)$ of the predictor approaches to a Dirac delta function $\delta$, in which case $\mu(\mathbf{x},\mathbf{s};\psi) \to f^{\phi}(\mathbf{x},\mathbf{s})$. Meanwhile, the additional shaping reward of the selector $\omega\sigma^2(\mathbf{x},\mathbf{s};\psi) \to 0$. Hence, our uncertainty-aware model degrades into the raw INVASE if the variance of all data points is infinitesimal. That corresponds to the condition in which every prediction is considered to be absolutely sure.

## 2 Proof of the Formula in Equation (7)

**Maximum Likelihood Estimation as minimizing KL Divergence** The Equation (6) is our optimization objective:

$$\psi^* = \arg\min_{\psi} E_{\mathbf{x}\sim P_D(\mathbf{x})}(d_{KL}(P_D(y|\mathbf{x},\mathbf{s})||P^{\psi}(y - f^{\phi}(\mathbf{x},\mathbf{s}))))\,.$$

The equivalence to maximum likelihood can be found in (Bishop 2006) as a ready-made theorem, which is omitted here for space limitations.

**Loss of Gaussian Maximum Likelihood Estimation** (Nix and Weigend 1994) provide a similar conclusion for common discriminative problems. In terms of our instance-wise feature selection problem:

$$\begin{aligned} l^{\phi}(\mathbf{x},\mathbf{s};\psi) &= -\log P_D^{\phi}(y|\mathbf{x},\mathbf{s};\psi) \\ &= -\log(\frac{1}{\sqrt{2\pi\sigma^2(\mathbf{x},\mathbf{s};\psi)}}\exp\,(-\frac{||y-\mu(\mathbf{x},\mathbf{s};\psi)||_2}{2\sigma^2(\mathbf{x},\mathbf{s};\psi)})) \\ &= \frac{\log\sigma^2(\mathbf{x},\mathbf{s};\psi)}{2} + \frac{||y-\mu(\mathbf{x},\mathbf{s};\psi)||_2}{2\sigma^2(\mathbf{x},\mathbf{s};\psi)} + \frac{\log 2\pi}{2} \\ &= \frac{\log\sigma^2(\mathbf{x},\mathbf{s};\psi)}{2} + \frac{||y-\mu(\mathbf{x},\mathbf{s};\psi)||_2}{2\sigma^2(\mathbf{x},\mathbf{s};\psi)} + constant\,. \end{aligned}$$

That is identical to Equation (7).

## 3 Pseudo-codes

Please refer to Algorithm 1.

## 4 Implementation Details

In practice, we append a 2-layer fully-connected 100-dimension branch to the predictor for computation of $\psi$, of which the shape and BatchNorm settings are consistent with the raw predictor.

*This work was done when Jia-Xing Zhong studied at Peking University.

Copyright © 2021, Association for the Advancement of Artificial Intelligence (www.aaai.org). All rights reserved.

**Algorithm 1** Training Process of Uncertainty-aware INVASE.

**Input:**
$\alpha$: learning rate of selector
$\beta$: learning rate of baseline network and predictor
$n$: batch size
$D$: dataset
$\omega$: a hyper-parametric weight for reward shaping
$\lambda$: a hyper-parametric weight for $l_1$-norm of feature dimensions
**Output:**
$\theta$: learned parameters of selector
$\phi$: learned parameters of predictor
$\gamma$: learned parameters of baseline network
$\psi$: learned parameters of uncertainty quantification

**repeat**
  Sample a mini-batch $(\mathbf{x}_j, y_j)_{j=1}^{n}$ from $D$
  **for** j=1,...,n **do**
    Compute selection probabilities: $\mathbf{p}_j = S^{\theta}(\mathbf{x}_j)$
    Obtain selection vector: $\mathbf{s}_j \sim Ber(\mathbf{x}_j)$
    Estimate loss difference:
    $\hat{l}(\mathbf{x}_j, \mathbf{s}_j) = -(\frac{\log \sigma^2(\mathbf{x}_j, \mathbf{s}_j; \psi)}{2} + \frac{||y_j - \mu(\mathbf{x}_j, \mathbf{s}_j; \psi)||_2}{2\sigma^2(\mathbf{x}_j, \mathbf{s}_j; \psi)}) - ||y - f^{\gamma}(\mathbf{x}_j)||_2)$
  Update the selector:
  $\theta = \theta - \alpha \frac{1}{n} \sum_{(\mathbf{x},y) \in batch} (\omega\sigma^2(\mathbf{x}, \mathbf{s}; \psi) - \hat{l}(\mathbf{x}, \mathbf{s}) - \lambda ||\mathbf{s}||_0) \nabla_{\theta} \log \pi_{\theta}(\mathbf{x}, \mathbf{s})$
  Update predictor with uncertainty quantification:
  $\phi = \phi - \beta \frac{1}{n} \sum_{(\mathbf{x},y) \in batch} \nabla_{\phi} l^{\phi}(\mathbf{x}, \mathbf{s}; \psi)$
  $\psi = \psi - \beta \frac{1}{n} \sum_{(\mathbf{x},y) \in batch} \nabla_{\psi} l^{\phi}(\mathbf{x}, \mathbf{s}; \psi)$
  Update baseline network:
  $\gamma = \gamma - \beta \frac{2}{n} \sum_{(\mathbf{x},y) \in batch} \mathbf{x}(f^{\gamma}(\mathbf{x}) - y)$
**until** Convergence

In terms of Equation (7), we have a term to optimize:

$$\frac{\log \sigma^2(\mathbf{x}, \mathbf{s}; \psi)}{2} + \frac{||y - \mu(\mathbf{x}, \mathbf{s}; \psi)||_2}{2\sigma^2(\mathbf{x}, \mathbf{s}; \psi)} .$$

However, that is numerically unstable: if $\sigma^2(\mathbf{x}, \mathbf{s}; \psi) = 0$, the second component $\frac{||y - \mu(\mathbf{x}, \mathbf{s}; \psi)||_2}{2\sigma^2(\mathbf{x}, \mathbf{s}; \psi)}$ will become infinite. Following (Kendall and Gal 2017), we actually utilize $\log \sigma^2$ as the computing unit. Therefore, the term is rewritten as:

$$\frac{\log \sigma^2(\mathbf{x}, \mathbf{s}; \psi)}{2} + \frac{1}{2} \exp(-\log \sigma^2(\mathbf{x}, \mathbf{s}; \psi)) \, ||y - \mu(\mathbf{x}, \mathbf{s}; \psi)||_2 .$$

## References


Bishop, C. M. 2006. *Pattern Recognition and Machine Learning*. Springer.

Kendall, A.; and Gal, Y. 2017. What uncertainties do we need in bayesian deep learning for computer vision? In *Advances in neural information processing systems*, 5574–5584.

Nix, D. A.; and Weigend, A. S. 1994. Estimating the mean and variance of the target probability distribution. In *Proceedings of 1994 IEEE International Conference on Neural Networks (ICNN'94)*, volume 1, 55–60 vol.1. ISSN null. doi:10.1109/ICNN.1994.374138.
